# Supplementary material for: Balancing Act: Constraining Disparate Impact in Sparse Models
Source: arXiv:2310.20673 source file (2024-03-08)
Supplement: Supplementary file 1 [file primal_param.tex]

\begin{table}[tbh!]
\centering
\resizebox{\columnwidth}{!}{%
\begin{tabular}{l|ccccccc}
\hline
\multirow{2}{*}{\textbf{Dataset}} &
  \multicolumn{1}{c|}{\multirow{2}{*}{\textbf{Task}}} &
  \multicolumn{1}{c|}{\multirow{2}{*}{\textbf{Initial step size}}} &
  \multicolumn{1}{c|}{\multirow{2}{*}{\textbf{Momentum}}} &
  \multicolumn{1}{c|}{\multirow{2}{*}{\textbf{Weight decay}}} &
  \multicolumn{1}{c|}{\multirow{2}{*}{\textbf{Scheduler}}} &
  \multicolumn{1}{c|}{\multirow{2}{*}{\textbf{Scheduler Milestones}}} &
  \multicolumn{1}{l}{\multirow{2}{*}{\textbf{Scheduler multiplier}}} \\
 &
  \multicolumn{1}{c|}{} &
  \multicolumn{1}{c|}{} &
  \multicolumn{1}{c|}{} &
  \multicolumn{1}{c|}{} &
  \multicolumn{1}{c|}{} &
  \multicolumn{1}{c|}{} &
  \multicolumn{1}{l}{} \\ \hline
\multirow{2}{*}{UTKFace} &
  Gender &
  1e-2 &
  0.9 &
  1e-4 &
  MultiStepLR &
  (60, 80, 90) &
  0.1 \\
 &
  Race &
  1e-2 &
  0.9 &
  1e-4 &
  MultiStepLR &
  (60, 80, 90) &
  0.1 \\ \hline
\multirow{2}{*}{FairFace} &
  Gender &
  1e-2 &
  0.9 &
  1e-4 &
  MultiStepLR &
  (60, 80, 90) &
  0.1 \\
 &
  Race &
  1e-2 &
  0.9 &
  1e-4 &
  MultiStepLR &
  (60, 80, 90) &
  0.1 \\ \hline
CIFAR &
  Class &
   &
   &
   &
   &
   &
   \\ \hline
\end{tabular}%
}
\caption{For a given dataset, we use the same \textbf{primal parameters} for all methods across sparsities. The milestones refer to the points (in \%) in the training procedure where it would be used.}
\label{tab:primal-table}
\end{table}
